# Supplementary material for: Few-shot Personalized Scanpath Prediction
Source: arXiv:2504.05499 source file (2025-04-07)
Supplement: Supplementary file 1 [file supp-loss.tex]

\begin{table}[h!]
    \centering
    \setlength{\tabcolsep}{2pt}  
    \resizebox{0.8\columnwidth}{!}{
    \begin{tabular}{p{4.0cm}p{1.0cm}p{1.0cm}p{1.0cm}}
        \toprule
        loss &  SM $\uparrow$ & MM $\uparrow$ & SED $\downarrow$ \\
        \midrule
        cls & 0.448 & 0.812 & 2.621 \\
        triplet & 0.442 & 0.812 & 2.400 \\
        Ours & 0.482 & 0.815 & 2.359 \\
        \bottomrule
    \end{tabular}}
    \vskip -0.1in
\caption{Loss ablation on COCO-Search18.\label{tab:supp-loss} } 
\end{table}
